# Supplementary material for: PrivacyRestore: Privacy-Preserving Inference in Large Language Models via Privacy Removal and Restoration
Source: arXiv:2406.01394 source file (2025-05-28)
Supplement: Supplementary file 1 [file Attack.tex]

\section{Detailed Implementation of Attack Methods}
\label{app:attack}
\subsection{Prompt injection Attack}
$d_\chi$-privacy injects noise into the original user inputs and transmits the garbled inputs to the server to protect the privacy spans.
We employ prompt injection attack to recover the initial question from the garbled inputs.
Following \citet{fbio2022ignore, xuchen2024sign}, we insert additional instructions before and after the user inputs to prompt the model to output the original user input rather than the normal response.
The template for the additional instructions is provided in Appendix \ref{app:prompt_PI}.

We set the maximum generation length for the prompt injection attack to 256 tokens. 
To evaluate the attack's performance, we calculate the ROUGE-L score between the generated output and the original user input.
A higher ROUGE-L score indicates greater overlap between the recovered text and the original input, signifying more successful attack results.

\subsection{Attribute inference attack}
Attribute inference attack attempts to steal user inputs by performing classification on the garbled inputs, where the target labels correspond to the token IDs of the original inputs. 
Since each input contains multiple tokens, this classification task is naturally a multi-label classification problem.
Following \citet{hao2022you}, we utilize a multi-layer perceptron (MLP) model as the classifier.
The input dimension is 4096 and the output dimension is the size of the whole vocabulary size.
To evaluate the attack's performance, we calculate the F1 score of the classification, where a higher F1 score indicates a more successful attack.
The attack targets can include garbled text from $d_\chi$-privacy, paraphrased text, or the meta vector from PrivacyRestore. 
The implementation details for text and vectors may vary slightly.

\textbf{Attribute inference attack on meta vector}.
To attack the meta vector from PrivacyRestore, we can directly use a fully-connected layer to transform the meta vector's dimension from $128\times K$ to the classifier's input dimension 4096.
We then perform classification on the transformed meta vector.

\textbf{Attribute inference attack on text}.
For garbled text from $d_\chi$-privacy or paraphrased text, we first transform the text into a vector representation. 
We utilize GPT-2 model \citep{radford2019language} to process the text input and obtain the last token's hidden state as the vector representation. 
Classification is then performed on this hidden state.

\subsection{Embedding inverse attack}
Different from attribute inference attack, embedding inverse attack steal the user inputs through the generative model to generate the original user inputs.
We utilize the GPT-2 model \citep{radford2019language} as the generative model and set the maximum generation length to 256.
We finetune the GPT-2 model on the training set for 20 epoch using the learning rate of 1e-5.
To evaluate the attack's performance, we compute the ROUGE-L score between the generated output of the GPT-2 model and the original user input, where higher scores indicate better attack effectiveness.
Similar to the attribute inference attack, the implementation of the embedding inverse attack differs between text and meta vectors.

\textbf{Embedding inverse attack on meta vector}. 
We use a fully-connected layer to transform the meta vector's dimension to the dimension of hidden state of GPT-2 model.
Then we directly input the transformed meta vector as the input embedding.

\textbf{Embedding inverse attack on text}.
We use Llama-2-chat-7b to process the text input and extract the last token's hidden state as the vector representation. 
This vector is then transformed by a fully connected layer to match the hidden state dimension of the GPT-2 model. 
Finally, it is fed into the GPT-2 model as the input embedding for subsequent generation.
