# Supplementary material for: PrivacyRestore: Privacy-Preserving Inference in Large Language Models via Privacy Removal and Restoration
Source: arXiv:2406.01394 source file (2025-05-28)
Supplement: Supplementary file 2 [file DP_DEF.tex]

\section{Formal Definitions of CDP and LDP}
\label{app:def_xDP}
\subsection{Centralized Differential Privacy (CDP)}
CDP protects individual privacy only \textbf{after data has been aggregated in a central repository}, which is defined as,
\begin{definition}
\textbf{(CDP).}
\label{def:CDP}
\textit{A randomized mechanism $\mathcal{M} : \mathcal{Q}\to\mathcal{G}$ fulfills $(\epsilon, \delta)$-differential privacy if for all adjacent queries $Q, Q^{\prime} \in \mathcal{Q}$ and all possible query results $G \subset \mathcal{G}$,}
\[
\mathbb{P}\left(\mathcal{M}(Q)\in G\right)\leq\exp(\epsilon)\mathbb{P}\left(\mathcal{M}(Q^{\prime})\in G\right)+\delta.
\]
\end{definition}
CDP \citep{cyn2016cali} ensures that adversaries cannot distinguish between $Q$ and $Q^\prime$ based on $G$ due to the similar probabilities, meaning the query results are probabilistically indistinguishable.
This prevents adversaries from inferring characteristics about the repository based on multiple queries and their results.

\subsection{Local Differential Privacy (LDP)}
However, privacy risks can also emerge during the data collection process itself, as attackers may intercept user inputs while they are being transmitted to the central repository.
LDP \citep{john2013local} protect user inputs \textbf{during transmission process} by ensuring that attackers cannot distinguish between any two adjacent inputs, which is defined as,
\begin{definition}
\textbf{(LDP).}
\label{def:LDP}
\textit{A randomized mechanism $\mathcal{M} : \mathcal{I}\to\mathcal{O}$ fulfills $(\epsilon, \delta)$-differential privacy if for all adjacent inputs $I, I^{\prime} \in \mathcal{I}$ and all possible outputs $O \subset \mathcal{O}$,}
\[
\mathbb{P}\left(\mathcal{M}(I)\in O\right)\leq\exp(\epsilon)\mathbb{P}\left(\mathcal{M}(I^{\prime})\in O\right)+\delta.
\]
\end{definition}
The mechanism $\mathcal{A}$ processes the user input before transmitting it. 
LDP ensures that, even if attackers intercept $O$, they cannot distinguish between the initial user input $I$ and the adjacent one $I^\prime$.
