# Supplementary material for: PrivacyRestore: Privacy-Preserving Inference in Large Language Models via Privacy Removal and Restoration
Source: arXiv:2406.01394 source file (2025-05-28)
Supplement: Supplementary file 3 [file addition_exp.tex]

\section{Additional Experiment Results}
\label{app:add_exp}
We report the additional experiment results on larger LLMs, such as Llama2-chat-13b \citep{touvron2023llama} and Llama3-8b-instruct \citep{llama3}.
As shown in Table \ref{app:table_avg_acc_13b} and Table\ref{app:table_avg_acc_8b}, PrivacyRestore can achieve comparable results to the normal inference and provide strong privacy preserving ability.

As shown Table \ref{app:table_gen_13b} and Table \ref{app:table_gen_8b}, with the model size of LLM increasing, the latency cost on Client is stable. 
The latency cost on the client is independent of the LLM size, and becomes more negligible when PrivacyRestore is applied to larger LLMs. 
Surprisingly, for Llama2-chat-13b on the Pri-NLICE dataset, PrivacyRestore can achieve 97\% of the initial throughput.
On average, PrivacyRestore can achieve 80\% of the initial throughput.

\begin{table*}
	\centering
        
	\resizebox{1\textwidth}{!}{
		\begin{tabular}{l   c cccc  cccc  cccc  cccc}
			\toprule
            % \cmidrule(lr){1-18}
            \multicolumn{17}{c}{\textbf{Pri-Ddxplus}} \\
            % \cmidrule(lr){1-18} 
            \midrule
		  \multirow{2}{*}{Methods} & \multirow{2}{*}{Privacy} &  \multicolumn{4}{c}{$\geq \text{Level 2}$} &  \multicolumn{4}{c}{$\geq \text{Level 3}$} &  \multicolumn{4}{c}{$\geq \text{Level 4}$} &  \multicolumn{4}{c}{$\geq \text{Level 5}$}\\ 
            \cmidrule(lr){3-18}
			& & MC1 $\uparrow$  & MC2 $\uparrow$ & ASR $\downarrow$ &  \multicolumn{1}{c|}{AF $\downarrow$}    &   MC1    & MC2  & ASR & \multicolumn{1}{c|}{AF}   &   MC1    & MC2  & ASR & \multicolumn{1}{c|}{AF} &   MC1 & MC2  & ASR & AF\\ 
            \midrule
            No Protection & $\times$ & 83.02 & 82.91 & 82.44 & \multicolumn{1}{c|}{35.06}
            & 83.02 & 82.91 & 82.44 & \multicolumn{1}{c|}{35.06}
            & 83.02 & 82.91 & 82.44 & \multicolumn{1}{c|}{35.06}
            & 83.02 & 82.91 & 82.44 & 35.06 \\

            Direct Removal  &\checkmark & 43.25 & 44.43 & 22.33 & \multicolumn{1}{c|}{25.94} 
            & 57.71 &57.31 & 4.13 &\multicolumn{1}{c|}{29.17} 
            &76.95 & 76.44 &0.06 &\multicolumn{1}{c|}{\textbf{0.93}} 
            &82.56 &82.17 &\textbf{0.00} &\textbf{0.00} \\

            DP \citep{qu2021natural} &\checkmark & 17.17 & 20.60 & 10.58 & \multicolumn{1}{c|}{23.18}
            & 7.17 & 20.60 & 10.58 & \multicolumn{1}{c|}{23.18}
            & 7.17 & 20.60 & 10.58 & \multicolumn{1}{c|}{23.18}
            & 7.17 & 20.60 & 10.58 & 23.18  \\

            DP on Privacy Spans &\checkmark & 54.09 &52.48 & 12.39 &\multicolumn{1}{c|}{18.44} 
            &61.07 &60.08 &7.48 &\multicolumn{1}{c|}{13.13} 
            &77.53 &76.43 &1.14 &\multicolumn{1}{c|}{2.71} 
            &82.37 &82.22 &\textbf{0.00} &5.78 \\

            \rowcolor{lightgray!45} 
            \textbf{Privacy Restoration}  &\checkmark & \textbf{90.57} & \textbf{88.86} & 12.45 & \multicolumn{1}{c|}{5.85}
            & \textbf{93.99} & \textbf{92.80} & 3.87 & \multicolumn{1}{c|}{5.50}
            & 85.21& \textbf{84.07}& \textbf{0.00}& \multicolumn{1}{c|}{3.98}
            & 82.31& 81.74& \textbf{0.00}& 0.90  \\

            \rowcolor{lightgray!45}
            w/o Top-K Heads Selector &\checkmark & 54.09 & 52.41 & 23.24 & \multicolumn{1}{c|}{56.81}
            & 57.45& 57.14& 2.17& \multicolumn{1}{c|}{82.23}
            & 77.53 & 75.91 & 0.06 & \multicolumn{1}{c|}{50.94}
            & 81.60& 81.33& \textbf{0.00} & 45.92  \\

            \rowcolor{lightgray!45}
            w/o Restoration Vectors Training &\checkmark & 18.59& 18.27 & 13.62 & \multicolumn{1}{c|}{5.85}
            & 37.83 & 38.83 & 3.80 & \multicolumn{1}{c|}{34.41}
            & 68.23 & 67.32 & 0.12 & \multicolumn{1}{c|}{39.72}
            & 81.34 & 81.01 & \textbf{0.00} & 9.05  \\

            \rowcolor{lightgray!45}
           w/o AWA &\checkmark &52.42 & 52.93 & \textbf{2.84} & \multicolumn{1}{c|}{\textbf{3.97}}
           & 80.50& 78.25 & \textbf{0.96} & \multicolumn{1}{c|}{\textbf{5.48}}
            & \textbf{85.60}& 83.59& \textbf{0.00} & \multicolumn{1}{c|}{38.86}
            & \textbf{82.69}& \textbf{82.36} & \textbf{0.00}& 5.55  \\

            \midrule 

            \multicolumn{17}{c}{\textbf{Pri-NLICE}} \\
            % \cmidrule(lr){1-18} 
            \midrule
		  \multirow{2}{*}{Methods} & \multirow{2}{*}{Privacy} &  \multicolumn{4}{c}{$\geq \text{Level 2}$} &  \multicolumn{4}{c}{$\geq \text{Level 3}$} &  \multicolumn{4}{c}{$\geq \text{Level 4}$} &  \multicolumn{4}{c}{$\geq \text{Level 5}$}\\ 
            \cmidrule(lr){3-18}
			&& MC1  & MC2 & ASR &  \multicolumn{1}{c|}{AF}    &   MC1    & MC2  & ASR & \multicolumn{1}{c|}{AF}   &   MC1    & MC2  & ASR & \multicolumn{1}{c|}{AF} &   MC1 & MC2  & ASR & F1\\ 
            \midrule
             No Protection & $\times$ & 81.56 & 78.37 & 91.54 & \multicolumn{1}{c|}{76.08}
            & 81.56 & 78.37 & 91.54 & \multicolumn{1}{c|}{76.08}
            & 81.56 & 78.37 & 91.54 & \multicolumn{1}{c|}{76.08}
            & 81.56 & 78.37 & 91.54 & 76.08 \\

            Direct Removal & \checkmark & 36.48 & 36.72 & \textbf{0.00} & \multicolumn{1}{c|}{\textbf{2.79}}
            & 43.43 & 46.36 & \textbf{0.00} & \multicolumn{1}{c|}{\textbf{0.43}}
            & 50.00 & 49.51 & \textbf{0.00} & \multicolumn{1}{c|}{0.15}
            & 53.15 & 52.00 & \textbf{0.00} & \textbf{0.00} \\

            DP \citep{qu2021natural} & \checkmark & 16.41 & 18.04 & \textbf{0.00} & \multicolumn{1}{c|}{32.01}
            & 16.41 & 18.04 & \textbf{0.00} & \multicolumn{1}{c|}{32.01}
            & 16.41 & 18.04 & \textbf{0.00} & \multicolumn{1}{c|}{32.01}
            & 16.41 & 18.04 & \textbf{0.00} & 32.01\\

            DP on Privacy Spans & \checkmark & 43.18 & 41.99 & 0.12 & \multicolumn{1}{c|}{56.68}
            & 59.59 & 56.59 &0.37 & \multicolumn{1}{c|}{35.36}
            & \textbf{67.42} & \textbf{64.50} & \textbf{0.00} & \multicolumn{1}{c|}{10.57}
            & \textbf{69.82} & \textbf{66.49} & \textbf{0.00} & 0.26 \\

            \rowcolor{lightgray!45} 
            \textbf{Privacy Restoration} & \checkmark & 79.92 & 75.36 & 0.88 & \multicolumn{1}{c|}{9.26}
            & 84.34 & 81.25 & 0.53 & \multicolumn{1}{c|}{2.01}
            & 65.15 & 64.08 & 0.12 & \multicolumn{1}{c|}{0.56}
            & 68.30 & 65.20 &\textbf{0.00}  & \textbf{0.00} \\

            \rowcolor{lightgray!45}
            w/o Top-K Heads Selector & \checkmark & 52.77 & 55.31 & 0.56 & \multicolumn{1}{c|}{22.54}
            & 71.33 & 69.47 & 0.45 & \multicolumn{1}{c|}{10.64}
            & 54.04 & 53.36 & 0.20 & \multicolumn{1}{c|}{1.44}
            & 56.31 & 54.13 & \textbf{0.00} & 0.14 \\

            \rowcolor{lightgray!45}
            w/o Restoration Vectors Training & \checkmark &46.46 & 47.81 & 0.41 & \multicolumn{1}{c|}{29.65}
            & 50.63& 51.88 & 0.35 & \multicolumn{1}{c|}{5.41}
            & 56.81 & 54.72 &0.14 & \multicolumn{1}{c|}{\textbf{0.11}}
            & 59.46 & 57.48 & \textbf{0.00} & 0.04 \\

            \rowcolor{lightgray!45}
           w/o AWA & \checkmark & \textbf{83.96} & \textbf{81.8} & 1.26 & \multicolumn{1}{c|}{33.54}
            & \textbf{84.59} & \textbf{81.45} & 0.97 & \multicolumn{1}{c|}{10.28}
            & 65.15 & 54.08 & 0.46 & \multicolumn{1}{c|}{5.76}
            & 68.30 & 65.20 & 0.02 & \textbf{0.00} \\
            
            \midrule

		\end{tabular}
  
	}

 \caption{
 Comparison of the model performance and the effectiveness of privacy protection among the compared methods on the Pri-Ddxplus and Pri-NLICE datasets on Llama2-chat-13b.
 The best model performance and privacy protection are marked in bold, excluding the No Protection method, as it does not provide any privacy protection.
}
\label{app:table_avg_acc_13b}
\end{table*}

\begin{table*}
	\centering
        
	\resizebox{1\textwidth}{!}{
		\begin{tabular}{l   c cccc  cccc  cccc  cccc}
			\toprule
            % \cmidrule(lr){1-18}
            \multicolumn{17}{c}{\textbf{Pri-Ddxplus}} \\
            % \cmidrule(lr){1-18} 
            \midrule
		  \multirow{2}{*}{Methods} & \multirow{2}{*}{Privacy} &  \multicolumn{4}{c}{$\geq \text{Level 2}$} &  \multicolumn{4}{c}{$\geq \text{Level 3}$} &  \multicolumn{4}{c}{$\geq \text{Level 4}$} &  \multicolumn{4}{c}{$\geq \text{Level 5}$}\\ 
            \cmidrule(lr){3-18}
			& & MC1 $\uparrow$  & MC2 $\uparrow$ & ASR $\downarrow$ &  \multicolumn{1}{c|}{AF $\downarrow$}    &   MC1    & MC2  & ASR & \multicolumn{1}{c|}{AF}   &   MC1    & MC2  & ASR & \multicolumn{1}{c|}{AF} &   MC1 & MC2  & ASR & AF\\ 
            \midrule
            No Protection & $\times$ & 43.38 & 44.87 & 99.67 & \multicolumn{1}{c|}{6.52}
            & 43.38 & 44.87 & 99.67 & \multicolumn{1}{c|}{6.52}
            & 43.38 & 44.87 & 99.67 & \multicolumn{1}{c|}{6.52}
            & 43.38 & 44.87 & 99.67 & 6.52 \\

            Direct Removal  &\checkmark & 28.34 & 29.68 & 39.83 & \multicolumn{1}{c|}{5.94} 
            & 32.34 &33.51 & 19.17 &\multicolumn{1}{c|}{4.39} 
            &42.47 & 44.24 &0.96 &\multicolumn{1}{c|}{1.61} 
            &\textbf{42.02} &\textbf{43.55} &0.38 &2.10 \\

            DP \citep{qu2021natural} &\checkmark & 22.14 & 23.84 & 99.74 & \multicolumn{1}{c|}{1.46}
            & 22.14 & 23.84 & 99.74 & \multicolumn{1}{c|}{1.46}
            & 22.14 & 23.84 & 99.74 & \multicolumn{1}{c|}{1.46}
            & 22.14 & 23.84 & 99.74 & 1.46  \\

            DP on Privacy Spans &\checkmark & 27.88 &29.39 & 97.86 &\multicolumn{1}{c|}{31.44} 
            &31.50 &32.10 &21.43 &\multicolumn{1}{c|}{8.61} 
            &40.54 &41.09 &1.61 &\multicolumn{1}{c|}{0.01} 
            &\textbf{42.02} &43.50 &1.22 &\textbf{0.00} \\

            \rowcolor{lightgray!45} 
            \textbf{Privacy Restoration}  &\checkmark & \textbf{76.56} & \textbf{78.02} & 23.49 & \multicolumn{1}{c|}{0.96}
            & \textbf{59.52} & 60.17 & 11.94 & \multicolumn{1}{c|}{1.10}
            & 54.48& \textbf{53.82}& \textbf{0.00}& \multicolumn{1}{c|}{\textbf{0.00}}
            & 40.67& 42.44& \textbf{0.00}& \textbf{0.00}  \\

            \rowcolor{lightgray!45}
            w/o Top-K Heads Selector &\checkmark & 31.37 & 30.79 & 81.14 & \multicolumn{1}{c|}{23.59}
            & 31.24& \textbf{62.34}& 5.03& \multicolumn{1}{c|}{\textbf{0.34}}
            & 44.54 & 44.38 & 0.77 & \multicolumn{1}{c|}{\textbf{0.00}}
            &41.83& 43.34& 0.19 & \textbf{0.00}  \\

            \rowcolor{lightgray!45}
            w/o Restoration Vectors Training &\checkmark & 21.62& 22.17 & 3.35 & \multicolumn{1}{c|}{\textbf{0.64}}
            & 19.69 &21.48 & \textbf{0.71} & \multicolumn{1}{c|}{1.05}
            &39.31 & 38.47 & 0.12 & \multicolumn{1}{c|}{0.98}
            & 41.63 & 43.34 & \textbf{0.00} & 0.61  \\

            \rowcolor{lightgray!45}
           w/o AWA &\checkmark &63.33 & 65.06 & \textbf{2.90} & \multicolumn{1}{c|}{5.81}
           &56.68& 57.64 & 12.65 & \multicolumn{1}{c|}{1.57}
            & \textbf{54.50}& 53.81& \textbf{0.00} & \multicolumn{1}{c|}{0.97}
            & 40.66&42.44 & \textbf{0.00}& 0.60  \\

            \midrule 

            \multicolumn{17}{c}{\textbf{Pri-NLICE}} \\
            % \cmidrule(lr){1-18} 
            \midrule
		  \multirow{2}{*}{Methods} & \multirow{2}{*}{Privacy} &  \multicolumn{4}{c}{$\geq \text{Level 2}$} &  \multicolumn{4}{c}{$\geq \text{Level 3}$} &  \multicolumn{4}{c}{$\geq \text{Level 4}$} &  \multicolumn{4}{c}{$\geq \text{Level 5}$}\\ 
            \cmidrule(lr){3-18}
			&& MC1  & MC2 & ASR &  \multicolumn{1}{c|}{AF}    &   MC1    & MC2  & ASR & \multicolumn{1}{c|}{AF}   &   MC1    & MC2  & ASR & \multicolumn{1}{c|}{AF} &   MC1 & MC2  & ASR & F1\\ 
            \midrule
             No Protection & $\times$ & 29.29 &28.35 & 55.80 & \multicolumn{1}{c|}{40.32}
            & 29.29 &28.35 & 55.80 & \multicolumn{1}{c|}{40.32}
            & 29.29 &28.35 & 55.80 & \multicolumn{1}{c|}{40.32}
            & 29.29 &28.35 & 55.80 & 40.32 \\

            Direct Removal & \checkmark & 16.03 & 16.92 & 10.2 & \multicolumn{1}{c|}{10.23}
            & 33.08 &30.93 & 7.42 & \multicolumn{1}{c|}{5.12}
            & 25.88 & 25.57 & 5.41 & \multicolumn{1}{c|}{\textbf{0.04}}
            & 26.01 & 25.83 & \textbf{0.00} & \textbf{0.00} \\

            DP \citep{qu2021natural} & \checkmark & 25.00 & 22.40 & 52.39 & \multicolumn{1}{c|}{12.87}
            & 25.00 & 22.40 & 52.39 & \multicolumn{1}{c|}{12.87}
            & 25.00 & 22.40 & 52.39 & \multicolumn{1}{c|}{12.87}
            & 25.00 & 22.40 & 52.39 & 12.87\\

            DP on Privacy Spans & \checkmark & 16.41 & 17.59 & 80.42 & \multicolumn{1}{c|}{\textbf{9.65}}
            & 25.50 & 24.85 & 76.13 & \multicolumn{1}{c|}{\textbf{1.01}}
            & 29.54 & 28.19 & 4.04 & \multicolumn{1}{c|}{0.45}
            & 28.66 &28.10 & \textbf{0.00} & 0.01 \\

            \rowcolor{lightgray!45} 
            \textbf{Privacy Restoration} & \checkmark & 93.81 & 94.50 & 33.58 & \multicolumn{1}{c|}{10.34}
            &\textbf{96.08} & \textbf{95.07} &6.81 & \multicolumn{1}{c|}{4.11}
            & \textbf{42.55} & \textbf{41.63} & \textbf{0.12} & \multicolumn{1}{c|}{0.06}
            & \textbf{38.76} & \textbf{37.97} & \textbf{0.00} & 0.01 \\

            \rowcolor{lightgray!45}
           w/o Top-K Heads Selector & \checkmark & 38.25 & 37.38 & 7.70 & \multicolumn{1}{c|}{15.87}
            & 43.30 & 41.85 & \textbf{3.28} & \multicolumn{1}{c|}{9.63}
            & 31.06 & 30.22 &0.63 & \multicolumn{1}{c|}{\textbf{0.04}}
            & 29.16 & 28.85 & \textbf{0.00} & \textbf{0.00} \\

            \rowcolor{lightgray!45}
            w/o Restoration Vectors Training & \checkmark & 26.26 & 26.58 & 90.90 & \multicolumn{1}{c|}{16.32}
            & 40.27 & 38.92 & 19.57 & \multicolumn{1}{c|}{5.69}
            & 27.39 & 26.90 & 0.25 & \multicolumn{1}{c|}{0.36}
            & 25.63 & 25.78 & \textbf{0.00} & \textbf{0.00} \\

            \rowcolor{lightgray!45}
           w/o AWA & \checkmark & \textbf{96.71} & \textbf{95.84} & \textbf{5.30} & \multicolumn{1}{c|}{23.75}
            & \textbf{96.08} & \textbf{95.07} & 6.69 & \multicolumn{1}{c|}{11.30}
            & \textbf{42.55} & \textbf{41.63} & \textbf{0.12} & \multicolumn{1}{c|}{0.75}
            & \textbf{38.76} & \textbf{37.97} & \textbf{0.00} & 0.05 \\
            
            \midrule

		\end{tabular}
  
	}

 \caption{
 Comparison of the model performance and the effectiveness of privacy protection among the compared methods on the Pri-Ddxplus and Pri-NLICE datasets on Llama3-8b-instruct. The best model performance and privacy protection are marked in bold, excluding the No Protection method, as it does not provide any privacy protection.
}
\label{app:table_avg_acc_8b}
\end{table*}

\begin{table*}
	\centering
        
	\resizebox{0.90\textwidth}{!}{
		\begin{tabular}{l   c  c c c c  c c }
			\toprule

            \multicolumn{8}{c}{\textbf{Pri-Ddxplus}} \\
            \midrule 
            \multirow{2}{*}{Methods}  & \multirow{2}{*}{Avg. Output Length} & \multirow{2}{*}{Latency on Server} & \multicolumn{4}{c}{Latency on Client} & \multirow{2}{*}{Throughput} \\
             \cmidrule(lr){4-7}
             & & & \multicolumn{1}{c|}{$\geq \text{Level 2}$}  
             & \multicolumn{1}{c|}{$\geq \text{Level 3}$} 
             & \multicolumn{1}{c|}{$\geq \text{Level 4}$}
             & $\geq \text{Level 5}$ &  \\
            \midrule
             Initial & 11.89 & 1232.52 & - & - & - & - & 9.65 \\
             \multirow{1}{*}{\textbf{Privacy Restoration}} & \multirow{1}{*}{8.16} &  1025.77 &  130.85 &  121.94 &  101.25 &  168.00 & \multirow{1}{*}{7.45 (\textbf{77\%})} \\
             % &  & \cellcolor{lightgray!45} & \cellcolor{lightgray!45} (15.44\%)
             % & \cellcolor{lightgray!45} (12.82\%) & \cellcolor{lightgray!45} (12.89\%) &
             % \cellcolor{lightgray!45} (19.49\%) &  & 
             \midrule

             \multicolumn{8}{c}{\textbf{Pri-NLICE}} \\
                \midrule 
            \multirow{2}{*}{Methods}  & \multirow{2}{*}{Avg. Output Length} & \multirow{2}{*}{Latency on Server} & \multicolumn{4}{c}{Latency on Client} & \multirow{2}{*}{Throughput} \\
             \cmidrule(lr){4-7}
             & & & \multicolumn{1}{c|}{$\geq \text{Level 2}$}  
             & \multicolumn{1}{c|}{$\geq \text{Level 3}$} 
             & \multicolumn{1}{c|}{$\geq \text{Level 4}$}
             & $\geq \text{Level 5}$ &  \\
            \midrule
             Initial & 5.83  & 953.35 & - & - & - & - & 6.12 \\
             \multirow{1}{*}{\textbf{Privacy Restoration}} & \multirow{1}{*}{5.83} &  848.14 &  104.46 &  98.18 &  86.42 &  88.01 & \multirow{1}{*}{5.97 (\textbf{97\%}}) \\
             % &  &  &  (15.24\%)
             % & \cellcolor{lightgray!45} (14.64\%) & \cellcolor{lightgray!45} (13.54\%) &
             % \cellcolor{lightgray!45} (13.53\%) &  & 

             \midrule
  
		\end{tabular}
	}
 \caption{Comparison of the generation efficiency on Llama2-chat-13b.  }
 \label{app:table_gen_13b}
\end{table*}

\newpage
\begin{table}[htbp]
	\centering
        
	\resizebox{0.90\textwidth}{!}{
		\begin{tabular}{l   c  c c c c  c c }
			\toprule

            \multicolumn{8}{c}{\textbf{Pri-Ddxplus}} \\
            \midrule 
            \multirow{2}{*}{Methods}  & \multirow{2}{*}{Avg. Output Length} & \multirow{2}{*}{Latency on Server} & \multicolumn{4}{c}{Latency on Client} & \multirow{2}{*}{Throughput} \\
             \cmidrule(lr){4-7}
             & & & \multicolumn{1}{c|}{$\geq \text{Level 2}$}  
             & \multicolumn{1}{c|}{$\geq \text{Level 3}$} 
             & \multicolumn{1}{c|}{$\geq \text{Level 4}$}
             & $\geq \text{Level 5}$ &  \\
            \midrule
             Initial & 63.70 & 1854.41 & - & - & - & - & 34.35 \\
             \multirow{1}{*}{\textbf{Privacy Restoration}} & \multirow{1}{*}{60.92} &  2290.97 &  105.07 &  94.85 &  85.00 &  139.10 & \multirow{1}{*}{25.41 (\textbf{74\%})} \\
             % &  & \cellcolor{lightgray!45} & \cellcolor{lightgray!45} (15.44\%)
             % & \cellcolor{lightgray!45} (12.82\%) & \cellcolor{lightgray!45} (12.89\%) &
             % \cellcolor{lightgray!45} (19.49\%) &  & 
             \midrule

             \multicolumn{8}{c}{\textbf{Pri-NLICE}} \\
                \midrule 
            \multirow{2}{*}{Methods}  & \multirow{2}{*}{Avg. Output Length} & \multirow{2}{*}{Latency on Server} & \multicolumn{4}{c}{Latency on Client} & \multirow{2}{*}{Throughput} \\
             \cmidrule(lr){4-7}
             & & & \multicolumn{1}{c|}{$\geq \text{Level 2}$}  
             & \multicolumn{1}{c|}{$\geq \text{Level 3}$} 
             & \multicolumn{1}{c|}{$\geq \text{Level 4}$}
             & $\geq \text{Level 5}$ &  \\
            \midrule
             Initial & 64  & 1983.10 & - & - & - & - & 32.27 \\
             \multirow{1}{*}{\textbf{Privacy Restoration}} & \multirow{1}{*}{64} &  2528.37 &  89.99 &  85.72 &  78.73 &  79.82 & \multirow{1}{*}{24.5 (\textbf{76\%}}) \\
             % &  &  &  (15.24\%)
             % & \cellcolor{lightgray!45} (14.64\%) & \cellcolor{lightgray!45} (13.54\%) &
             % \cellcolor{lightgray!45} (13.53\%) &  & 

             \midrule
  
		\end{tabular}
	}
 \caption{Comparison of the generation efficiency on Llama2-chat-8b. }
 \label{app:table_gen_8b}
\end{table}
