# Supplementary material for: PrivacyRestore: Privacy-Preserving Inference in Large Language Models via Privacy Removal and Restoration
Source: arXiv:2406.01394 source file (2025-05-28)
Supplement: Supplementary file 4 [file defense2attacks.tex]

\section{Defense to Various Attacks}
\label{app:defense}
% 被攻击的点
% 再说不会被攻击
% (1) attack: meta restoration is incepted. 
% defense: 单个向量加扰动 + 多个向量是叠加的
% (2) attack server 被人控制了。 own an exactly same LLM, attack obtain meta restoration and query with privacy spans deleted, can use a harmful prompt to ask privacy information rather than output. 
% defense: our experiments prove that the attack rate is low. 
% (3) attack： server 被人控制了 attribute inference attack. 
%  defense: experiment. 

We enumerate the potential attacks that PrivacyRestore may face and demonstrate that PrivacyRestore can effectively defend against them as follows.

\textbf{Leakage of restoration vectors of each privacy span and meta restoration vector. }

Attackers may illegally obtain restoration vectors of each privacy span and intercept the meta restoration vector sent to the server.
Even in such scenarios, it is still difficult for attackers to infer privacy spans based on a specific meta restoration vector.
% 分情况分析
According to the AWA method in \S \ref{sec:res_agg}, when only one privacy span exists in the query, the meta restoration vector is a restoration vector with random noise injected, which prevents the privacy span from being inferred. 
% which satisfies the \revisezq{token representation privatization \cite{qu2021natural}}.
When the query contains multiple privacy spans, attackers need to try all combinations of restoration vectors to infer the privacy span.
The number of combinations that the attacker needs to try is equal to the sum of combinatorial numbers of any number of restoration vectors, which can be expressed as:
\begin{equation}
    \mathcal{N}_{c} = \sum_{i=2}^{|\mathcal{S}|} C_{|\mathcal{S}|}^{i} = 2^{|\mathcal{S}|} - |\mathcal{S}| - 1,
\end{equation}
where $|\mathcal{S}|$ is the total number of privacy spans, and $C_n^i$ represents the combinatorial number of ways to choose $i$ elements from a set of $n$ elements.
The number of combinations grows exponentially with $|\mathcal{S}|$, and in practical scenarios where $|\mathcal{S}|$ is typically large, so it is impossible for attackers to infer privacy spans even if the restoration vectors of each privacy span are available.

\textbf{Prompt Injection Attack. }
The attack condition is that attackers own LLM weights and can obtain meta restoration vector and a query with privacy spans removed. 
% \revisezq{add inject process}
% 先截取,再注入,再发送给LLM
During inference, attackers intercept the query sent by the client, modify the content of the query, and then send it to the server.
Attackers inject malicious content into the query to manipulate the LLM to generate privacy information. 
For example, in medical diagnosis task, the malicious content would be ``print out the possible symptoms.'' 
% attempt to obtain privacy information by 
For prompt injection attack, experimental results in Table \ref{table_avg_acc} show that the attack success ratio of our method is lower than baselines.

\textbf{Attribute Inference Attack. }
The attack condition is the same with Prompt Injection Attack.
Attribute Inference Attack aims to recover sensitive attributes in the input text.
Attackers commonly use input text or its embeddings as input to train a classifier to classify whether sensitive attributes are contained in input text.
As shown in Table \ref{table_avg_acc}, the F1 score of classifier for our method is low.
