# Supplementary material for: PrivacyRestore: Privacy-Preserving Inference in Large Language Models via Privacy Removal and Restoration
Source: arXiv:2406.01394 source file (2025-05-28)
Supplement: Supplementary file 5 [file implementation_details.tex]

\section{Implementation Details.}
\label{app:imple_detail}
% \textbf{Implementation details.}
For the fine-tuning process described in \S \ref{sec:res_corr}, we only train the restoration vectors and fix all other parameters of LLM. 
The training is conducted for five epochs with a batch size of 8. 
This process takes 4\textasciitilde5 hours on a single A100 GPU, which is a reasonable duration for retraining the model when new privacy spans are introduced. 
% We set the learning rate as 1e-04 with 0.001 weight decay. 
% We use the cosine learning rate scheduler with 0 warmup ratio.

For the classifier used in the attribute inference attack, we employ a 2-layer Multilayer Perceptron (MLP) as the classifier, following the approach in \cite{Li2022perna}.
The classifier is trained on the same dataset used for restoration vector training. 
The classifier takes the query representation as the input and predicts whether the query contain specific symptoms. 
We regard the meta restoration vector as the query representation. 
The other methods in \S \ref{sec:baseline} do not have obvious representations associated with the privacy spans. 
We utilize the hidden state of the last token from the last layer of LLM as the query representation. 
% We training the classifiers for ten epochs using a batch size of 32. 
% We set the learning rate as 3e-5 with no weight decay. 
% We use the linear learning rate scheduler with 100 warmup steps.
% \revisezq{mention training data of attribute inference.}

Differential privacy \citep{qu2021natural} use $\eta$ to control the strength of injected noise.
Smaller $\eta$ provides stronger privacy protection but results in significant performance degradation.
%As shown in \cite{li2023privacy}, the range of $\eta$ is from 75 to 175 for acceptable performance degradation .
%For DP based baseline in Section \ref{sec:baseline}, we set the $\eta$ to 75 considering better privacy protection. 
As shown in \cite{li2023privacy}, $\eta$ ranges from 75 to 175. A lower value represents a higher level of privacy protection. 
For the DP based methods, we set $\eta$ to 75 to prioritize privacy protection.
% \revisezq{why 75, following any paper? what is the range of $\eta$?}
For noise injection regarding the single restoration vector case mentioned in \S \ref{sec:res_agg}, we use the same $\eta=75$ to maintain a consistent noise level.

To evaluate inference efficiency, we use the greedy search decoding strategy and restrict the max generation length to 64.
For top-K heads selector, we following the setting of \cite{li2023iti} and set K to 48.
All of our experiment is conducted on the NVIDIA A800.
