# Supplementary material for: PrivacyRestore: Privacy-Preserving Inference in Large Language Models via Privacy Removal and Restoration
Source: arXiv:2406.01394 source file (2025-05-28)
Supplement: Supplementary file 6 [file noweight.tex]

\subsection{Attention-aware Weighted Aggregation vs Equal Weighted Aggregation}
\label{app:awa}
In order to verify the effectiveness of Attention-aware Weighted Aggregation (AWA) component, we compare the performance and the inference efficiency between equal weighted aggregation and attention-aware weighted aggregation.
Different from attention-aware weighted aggregation, equal weighted aggregation computes the meta vector by simply summing up all restoration vectors.

As shown in Table \ref{tbl:no_weight}, the MC1, MC2, ROUGE-L, and LLM-J scores of equal weighted aggregation are all lower than those of attention-aware weighted aggregation, indicating that simply summing all restoration vectors equally degrades performance.
This degradation is primarily due to the equal weights diluting the influence of critical spans while amplifying the effect of irrelevant ones.
In terms of inference efficiency, the throughput difference between Attention-Aware Weighted Aggregation and Equal Weighted Aggregation is minimal. 
This suggests that the weight computation, as defined in Eq \ref{eq:weight}, is efficient and does not significantly impact overall throughput.

\begin{table*}[!htbp]
	\centering
        
		\resizebox{0.98\textwidth}{!}{
	   \begin{tabular}{ l l |  ccccc  }
	   \toprule
           Datasets & Methods  & MC1 $\uparrow$ & MC2 $\uparrow$ & ROUGE-L $\uparrow$ & LLM-J $\uparrow$ & TP $\uparrow$ \\
            % \midrule
            \cmidrule(lr){1-7} 
            \multirow{2}{*}{Pri-DDXPlus} & Equal Weighted Aggregation & 53.84 & 51.12 & 26.32 & 4.29 & \textbf{26.35}    \\
            ~ & Attention-aware Weighted Aggregation & \textbf{62.97} & \textbf{60.19} & \textbf{27.24} & \textbf{4.47} & 26.09 \\

            \cmidrule(lr){2-7} 
            \multirow{2}{*}{Pri-NLICE} & Equal Weighted Aggregation & 46.92 & 45.89 & 22.78 & 3.12 & \textbf{32.75} \\
            ~ & Attention-aware Weighted Aggregation & \textbf{62.23} & \textbf{57.94} & \textbf{24.42} & \textbf{3.67} & 32.33 \\

            \cmidrule(lr){2-7} 
            \multirow{2}{*}{Pri-SLJA} & Equal Weighted Aggregation & 30.88 & 30.70 & 30.96 & 4.10 & \textbf{31.00} \\
            ~ & Attention-aware Weighted Aggregation & \textbf{35.47} & \textbf{35.41} & \textbf{37.56} & \textbf{5.25} & 30.73 \\

                \midrule

		\end{tabular}
  
	}

    \vspace{-0.5em}
 \caption{
Comparison of the performance and the inference efficiency between Equal Weighted Aggregation and Attention-aware Weighted Aggregation. 
The best results are highlighted in \textbf{bold}.
}
\label{tbl:no_weight}
\end{table*}
