# Supplementary material for: PrivacyRestore: Privacy-Preserving Inference in Large Language Models via Privacy Removal and Restoration
Source: arXiv:2406.01394 source file (2025-05-28)
Supplement: Supplementary file 7 [file proof_1.tex]

\textbf{Proof of $d_\chi$-privacy}. 
As shown in Definition \ref{def:dx_privacy}, if the input length is 1, indicating a single token $i_1$, $d_\chi$ can be:
\[
\mathbb{P}\left(\mathcal{M}(i_1)\in o_1 \right)\leq\exp(\epsilon d_\chi(i_1, i_1^\prime))\mathbb{P}\left(\mathcal{M}(i_1^{\prime})\in o_1\right),
\]
where $o_1$ is the possible output set for $\mathcal{M}(i_1)$ and the privacy budget is $\epsilon d_\chi(i_1, i_1^\prime)$.
When the input becomes the sequential tokens $I = \{i_1, i_2, ..., i_n\}$ with corresponding output sets $O = \{o_1, ..., o_n \}$, the LCP for the sequence of length $n$ is:

% \begin{align*}
% \notag
%     \mathbb{P}&\left(\mathcal{M}(I)\in O\right) \\
%     &= \mathbb{P}\left(\mathcal{M}(i_1)\in o_1\right) \cdot 
%     \mathbb{P}\left(\mathcal{M}(i_2)\in o_2\right) \cdot 
%     ...  \cdot \mathbb{P}\left(\mathcal{M}(i_n)\in o_n \right) 
%     \notag
%     \\&\leq [\exp(\epsilon d_\chi(i_1, i_1^\prime))\mathbb{P}\left(\mathcal{M}(i_1^{\prime})\in o_1\right)] \cdot ... \\
%     & \qquad ... \cdot [\exp(\epsilon d_\chi(i_n, i_n^\prime))\mathbb{P}\left(\mathcal{M}(i_n^{\prime})\in o_n\right)]  
%     \notag
%     \\&= \exp[\epsilon (
%     d_\chi(i_1, i_1^\prime) + \cdots + d_\chi(i_n, i_n^\prime)
%     )]\mathbb{P}\left(\mathcal{M}(I^{\prime})\in O\right) 
%     \notag
%     \\&= \exp[ \epsilon
%     \sum_{j=0}^n d_\chi(i_j, i_j^\prime)
%     ]
%     \mathbb{P}\left(\mathcal{M}(I^{\prime})\in O\right),
% \end{align*}
\vspace{-5px}
\begin{align*}
\mathbb{P}&\left(\mathcal{M}(I)\in O\right) \\
    &= \mathbb{P}\left(\mathcal{M}(i_1)\in o_1\right) \cdot 
    \mathbb{P}\left(\mathcal{M}(i_2)\in o_2\right) \cdot \\
    &\qquad \qquad ... \cdot 
    \mathbb{P}\left(\mathcal{M}(i_n)\in o_n \right) 
    \notag
    \\&\leq [\exp(\epsilon d_\chi(i_1, i_1^\prime)) \mathbb{P}\left(\mathcal{M}(i_1^{\prime})\in o_1\right)] \cdot 
    \\&\qquad \qquad ... \cdot 
    [\exp(\epsilon d_\chi(i_n, i_n^\prime)) \mathbb{P}\left(\mathcal{M}(i_n^{\prime})\in o_n\right)]  
    \notag
    \\&= \exp\Big[\epsilon \big(
    d_\chi(i_1, i_1^\prime) + 
    \\& \qquad \qquad... + d_\chi(i_n, i_n^\prime)
    \big)\Big]
    \mathbb{P}\left(\mathcal{M}(I^{\prime})\in O\right) 
    \notag
    \\&= \exp\Big[ \epsilon
    \sum_{j=0}^n d_\chi(i_j, i_j^\prime)
    \Big]
    \mathbb{P}\left(\mathcal{M}(I^{\prime})\in O\right),
\end{align*}

where the privacy budget is $\epsilon \sum_{j=1}^nd_\chi(i_j, i_j^\prime)$.
Commonly, we use the Euclidean distance as the $d_\chi$ function and obviously $\sum_{j=1}^nd_\chi(i_j, i_j^\prime) \propto n$. 
Therefore, the privacy budget of LDP grows linearly with the length $n$.

\textbf{Proof of LDP}. 
As stated in Definition \ref{def:LDP}, if the length of input is 1, corresponding to a single token $i_1$, LDP can be expressed as:
\[
\mathbb{P}\left(\mathcal{M}(i_1)\in o_1 \right)\leq\exp(\epsilon)\mathbb{P}\left(\mathcal{M}(i_1^{\prime})\in o_1\right)+\delta,
\]
where $o_1$ is the possible output set of $\mathcal{M}(i_1)$ and the privacy budget is controlled by $(\epsilon, \delta)$.
Considering the sequence tokens $I = \{i_1, i_2, ..., i_n\}$ and corresponding output sets $O = \{o_1, o_2, ..., o_n\}$, the CDP for the sequence of length $n$ can be written as: 

% \begin{align*}
%     \mathbb{P}\left(\mathcal{M}(I)\in O \right) &= \mathbb{P}\left(\mathcal{M}(i_1)\in o_1 \right) \cdot \mathbb{P}\left(\mathcal{M}(i_2)\in o_2 \right) \cdot  \\
%     & \quad ... \cdot \mathbb{P}\left(\mathcal{M}(i_n)\in o_n \right) \\
%     &\leq [\exp(\epsilon)\mathbb{P}\left(\mathcal{M}(i_1^{\prime})\in o_1\right)+\delta]
%     \cdot \\
%     & \quad ... \cdot [\exp(\epsilon)\mathbb{P}\left(\mathcal{M}(i_n^{\prime})\in o_n\right)+\delta] \\ 
%     &= \exp(n\epsilon)\mathbb{P}\left(\mathcal{M}(I^{\prime})\in O\right) + \\
%     & \delta \cdot 
%     \sum_{i=1}^{n} \prod_{j!=i} \mathbb{P}\left(\mathcal{M}(i_j^{\prime})\in o_j\right) 
%     + \delta^2 \cdot ...,
% \end{align*}

\begin{align*}
    \mathbb{P}&\left(\mathcal{M}(I)\in O \right) \\
    &= \mathbb{P}\left(\mathcal{M}(i_1)\in o_1 \right) \cdot 
    \mathbb{P}\left(\mathcal{M}(i_2)\in o_2 \right) \cdot \\
    &\qquad \qquad ... \cdot 
    \mathbb{P}\left(\mathcal{M}(i_n)\in o_n \right) \\
    &\leq [\exp(\epsilon) \mathbb{P}\left(\mathcal{M}(i_1^{\prime})\in o_1\right) + \delta] 
    \cdot \\
    &\qquad \qquad ... \cdot 
    [\exp(\epsilon) \mathbb{P}\left(\mathcal{M}(i_n^{\prime})\in o_n\right) + \delta] \\ 
    &= \exp(n\epsilon) \mathbb{P}\left(\mathcal{M}(I^{\prime})\in O\right)  \\
    &\qquad \qquad + \delta \cdot 
    \sum_{i=1}^{n} \prod_{j \neq i} \mathbb{P}\left(\mathcal{M}(i_j^{\prime})\in o_j\right) + \delta^2 \cdots,
\end{align*}

where $\delta$ is typically considered a very small value. 
When $\delta$ approaches 0, we consider only the first two terms and then, 
\begin{align*}
    \mathbb{P}\left(\mathcal{M}(I)\in O \right) &\leq \exp(n\epsilon)\mathbb{P}\left(\mathcal{M}(I^{\prime})\in O\right) \\
    &+ \delta \cdot 
    \sum_{i=1}^{n} \prod_{j!=i} \mathbb{P}\left(\mathcal{M}(i_j^{\prime})\in o_j\right),
\end{align*}
which indicating the privacy budget becomes $\big(n\epsilon, \delta \cdot \sum_{i=1}^{n} \prod_{j!=i} \mathbb{P}\left(\mathcal{M}(i_j^{\prime})\in o_j\right) \big)$, according to the Definition of LDP in Section \ref{def:LDP} .
The first term $n \epsilon$ obviously grows linearly with the length $n$.
The second term can be view as $\delta$ multiplied by $\sum_{i=1}^{n} \prod_{j!=i} \mathbb{P}\left(\mathcal{M}(i_j^{\prime})\in o_j\right)$.
The second term summarizes $n$ multiplicative terms, each bounded within $(0, 1)$. 
The second term can be approximately considered to grow linearly with $n$. 
Therefore, the privacy budget of CDP also grows linearly with the length $n$.

\textbf{Proof of CDP}. The definition of CDP, as shown in Section \ref{def:CDP}, is similar to LDP,  with the only difference being that CDP applies to the user query $Q = \{q_1, q_2, ..., q_n\}$ rather than the text input $I = \{i_1, i_2, ..., i_n\}$.
If we consider the token $i_n$ as a sub-query $q_n$,
then similarly the definition of CDP for sequential sub-queries $Q = \{q_1, q_2, ..., q_n\}$ can be:
\begin{align*}
\mathbb{P}\left(\mathcal{M}(Q)\in G \right) &\leq \exp(n\epsilon)\mathbb{P}\left(\mathcal{M}(Q^{\prime})\in G\right) 
\\ &+ \delta \cdot \sum_{i=1}^{n} \prod_{j!=i} \mathbb{P}\left(\mathcal{M}(q_j^{\prime})\in g_j\right),
\end{align*}
where $G = \{g_1, g_2, ..., g_n\}$ are the possible output sets for sequence inputs $Q$. The privacy budget is $\big( n\epsilon, \delta \cdot \sum_{i=1}^{n} \prod_{j!=i} \mathbb{P}\left(\mathcal{M}(q_j^{\prime})\in g_j\right) \big)$ and also grows linearly with the length $n$.
