# Supplementary material for: PrivacyRestore: Privacy-Preserving Inference in Large Language Models via Privacy Removal and Restoration
Source: arXiv:2406.01394 source file (2025-05-28)
Supplement: Supplementary file 8 [file EWA_vs_AWA.tex]

% \subsection{The Effectiveness of Attention-Aware Weighted Aggregation (AWA)}
% \label{app:EWAvsAWA}
% To assess the effectiveness of the Attention-Aware Weighted Aggregation (AWA) component, we compare its performance and inference efficiency against Equal Weighted Aggregation (EWA). Unlike AWA, EWA generates the meta vector by summing all restoration vectors equally. 

% As shown in Table \ref{tbl:no_weight}, EWA results in lower MC1, MC2, ROUGE-L, and LLM-J scores compared to AWA, indicating that equal weighting diminishes performance by diluting critical spans and amplifying irrelevant ones. The inference efficiency of AWA and EWA is comparable, as the weight computation in Eq \ref{eq:weight} has minimal impact on throughput. 
% % \input{fig/tables/weight_table}
