# Supplementary material for: PrivacyRestore: Privacy-Preserving Inference in Large Language Models via Privacy Removal and Restoration
Source: arXiv:2406.01394 source file (2025-05-28)
Supplement: Supplementary file 10 [file representation_engineering.tex]

\revisejy{\section{Supplement to Related Work}
\label{app:representation_engineering}
\subsection{Representation Engineering}
Representation Engineering, introduced by \citep{Zou2023RepresentationEA}, uses difference vectors between activations on an individual stimuli to capture representations of a concept. Adjusting the neural activations of the model at the inference time to align with or diverge from these directions effectively modulates the semantic properties of its responses. Methods based on Representation Engineering\citep{li2023iti, hernandez2023inspecting,chen2024truth,turner2023activation} directly add multiples of a concept direction to neural activation to perform knowledge editing. Nonetheless, these efforts have made significant progress at the knowledge editing level, but no one before us had systematically applied this technology to privacy protection in large language models.}

% \subsubsection{Attention Mechanism}
