# Supplementary material for: PrivacyRestore: Privacy-Preserving Inference in Large Language Models via Privacy Removal and Restoration
Source: arXiv:2406.01394 source file (2025-05-28)
Supplement: Supplementary file 11 [file dataset_construct_copy.tex]

\section{Datasets}
\label{app:dataset}
\subsection{Definitions of Privacy Level}
\label{app:level}
We classify the privacy of patients' symptoms into five levels, with higher levels indicating greater sensitivity.
The detail definitions of privacy level are present in Table \ref{tbl:privacy_level}.
We also display the distribution of symptoms across five privacy levels on Pri-Ddxplus dataset and Pri-NLICE dataset.

\begin{table}[h]
{
\def\arraystretch{1.1}
\begin{tabularx}{\linewidth}
{ >{\setlength\hsize{.15\hsize}} X >{\setlength\hsize{0.75\hsize}} X r }
\toprule
\textbf{Privacy Level} & \textbf{Definition}                                                       & \textbf{\%} \\ \midrule
\textbf{Level 1} & \texttt{Public information, symptoms or antecedents that are common, widely known, and do not reveal any personal or sensitive information. Examples include sneezing, headache, or minor injuries.}  & $20.43$ \\
\textbf{Level 2} & \texttt{Non-sensitive personal information, symptoms or antecedents that may be personal but not necessarily sensitive or revealing. These may include common illnesses like cold or flu, allergies, or minor digestive issues.}  & $22.58$ \\
\textbf{Level 3} & \texttt{Potentially sensitive information, symptoms or antecedents that could be indicative of underlying health conditions but are not immediately sensitive or stigmatizing. Examples include chronic conditions like diabetes, hypertension, or asthma.}  & $40.86$ \\
\textbf{Level 4} & \texttt{Sensitive personal information, symptoms or antecedents that may be stigmatizing or have social implications if disclosed publicly. This could include mental health issues like depression or anxiety, reproductive health concerns, or substance abuse.}  & $6.98$ \\
\textbf{Level 5} & \texttt{Highly sensitive information, symptoms or antecedents that are highly personal, stigmatizing, or potentially life-altering if disclosed publicly. This category includes sexually transmitted infections, HIV/AIDS, certain types of cancer, or rare and serious medical conditions.}  & $9.13$ \\
\bottomrule
\end{tabularx}
}
\caption{The definition of different Privacy Level for possible symptoms in PriDdxplus. 
The rightmost column displays the ratio of symptoms at the corresponding privacy level.}
\label{tbl:privacy_level} 
\end{table}

\subsection{Construction Process}
\label{app:construction}
We utilized GPT-3.5 \citep{ouyang2022training} to assess the privacy levels of all possible symptoms in Ddxplus \citep{ars2022ddxplus} and NLICE \cite{al2023nlice}, ranging from non-sensitive to highly sensitive. 
The assessing prompt template is shown in Figure \ref{fig:privacy_level}.

We also assign each sample three random pathologies as incorrect diagnoses to combine with the correct diagnosis and create options. Some data samples are present in Figure \ref{fig:example}.

The initial Ddxplus \citep{ars2022ddxplus} and NLICE \citep{al2023nlice} dataset is extensive, and we observed that for most samples, providing only non-sensitive symptoms often yields diagnosis outputs similar to those obtained when intact symptoms are provided.
Privacy preserving for these samples is meaningless because users can directly hide those privacy spans and obtain approximate diagnosis results.
In real world, sensitive symptoms sometimes play an vital role in diagnosis and privacy preserving is highly valuable.
Our dataset is designed to benchmark various privacy-preserving methods and must include samples where privacy symptoms are crucial for diagnosis outcomes.
We utilize the KL divergences to measure the importance degree of privacy spans.
We calculate the KL divergence between the model output distributions with and without the privacy symptoms included.
Higher KL divergence indicates that the absence of sensitive symptoms may lead to different or even incorrect output.
After filtering, we obtain the Pri-Ddxplus and Pri-NLICE dataset for privacy preserving.

\begin{figure*}[htbp]
\centering
\includegraphics[width=1\textwidth]{fig/privacy_level.pdf}
\caption{
The prompt used for privacy level assessing.
}
\label{fig:privacy_level}
\end{figure*}

\begin{figure*}[htbp]
\centering
\includegraphics[width=1\textwidth]{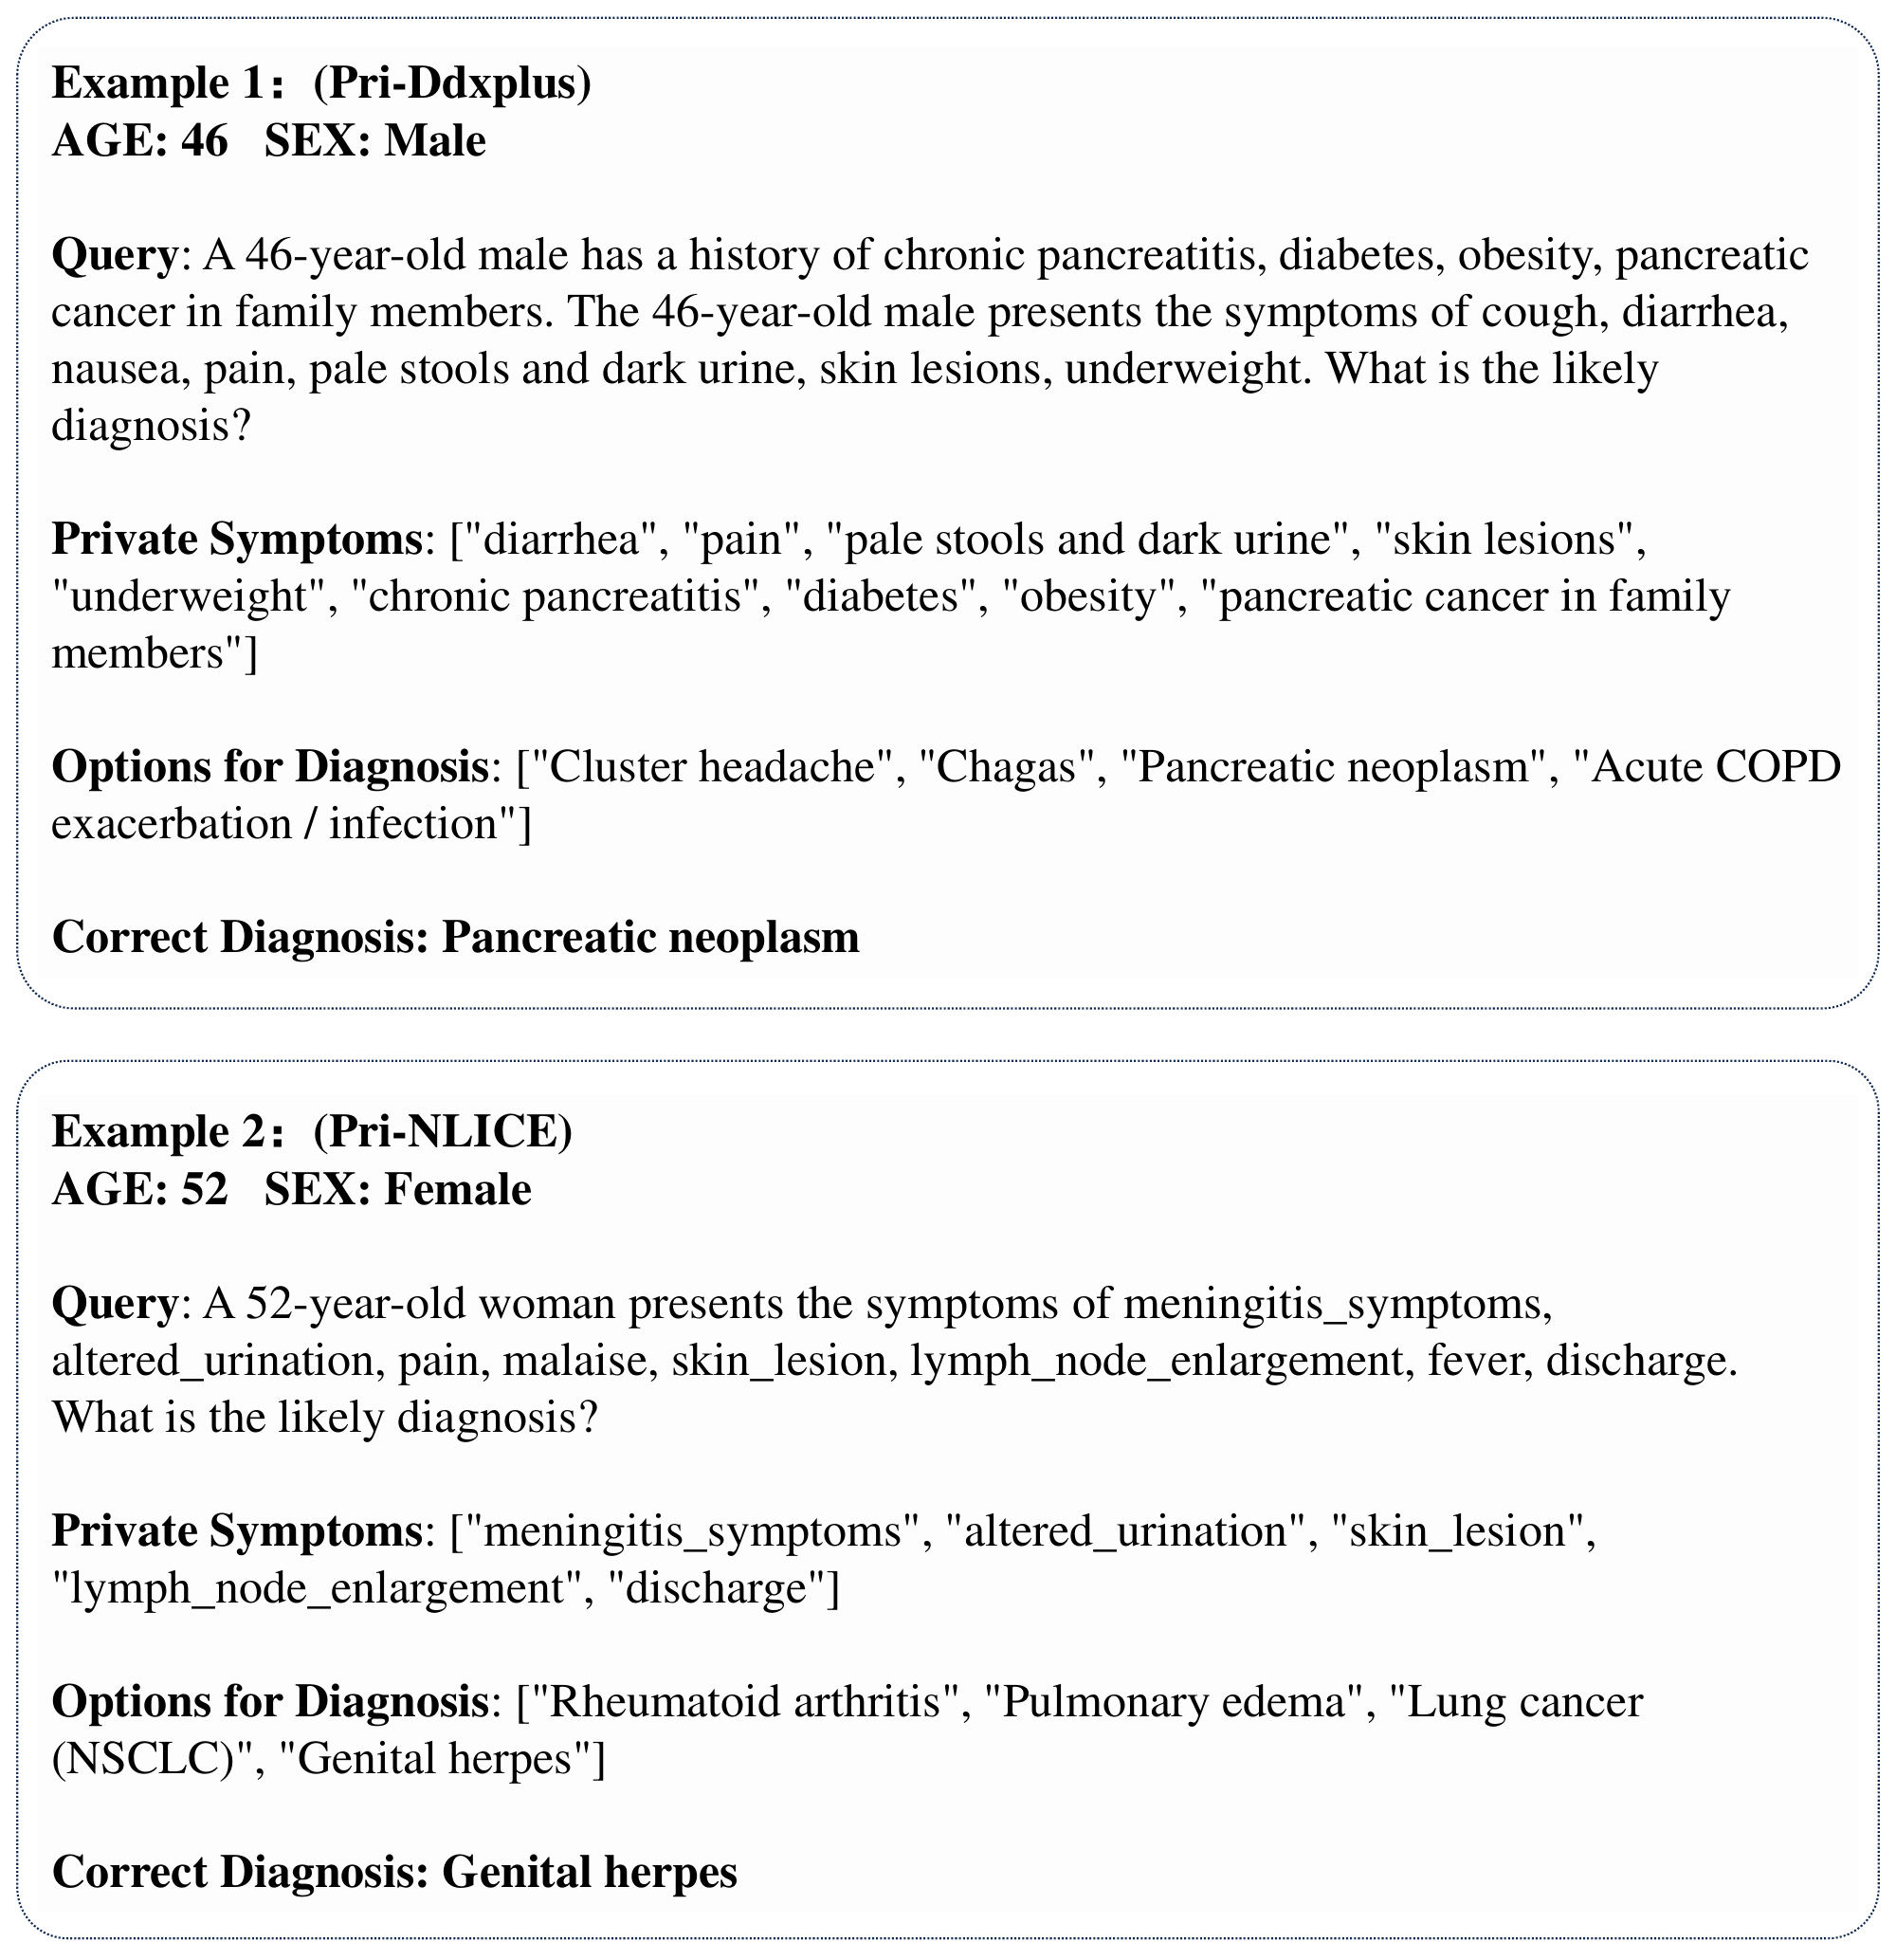}
\caption{
Some data examples in Pri-Ddxplus and Pri-NLICE datasets.
}
\label{fig:example}
\end{figure*}

\subsection{Statistical Information}
\label{sec:dataset}
We show the statistics of the obtained Pri-Ddxplus and Pri-NLICE dataset in Table \ref{tbl:statistics}. 
We tally the number of instances, symptom types, and diagnosis types.
Symptoms with a privacy level greater than 2 were considered private.
We calculate the number of privacy symptom types, which are regarded as privacy spans.
We also compute the average occurrence of privacy symptoms per instance.

Pri-Ddxplus commonly contains more instances and more privacy symptoms types compared to Pri-NLICE.
Each sample in Pri-Ddxplus contains six privacy symptoms on average, while samples in Pri-NLICE have four privacy symptoms.

\begin{table}[H]
    \centering
    \def\arraystretch{1.5}
    \resizebox{0.95\textwidth}{!}{
        \begin{tabular}[h]{ccccccc}
            \hline
            \multicolumn{7}{c}{\textbf{Pri-Ddxplus}} \\
          \hline
           {\textbf{Dataset Split}} &  {\textbf{Instances}} & {\textbf{Symptom Type}} & {\textbf{Diagnosis Type}} & {\textbf{Privacy Symptom Type}} &
          {\textbf{Avg. Privacy Symptoms}}\\
          \hline
          \textbf{All} & 7509& 187 &73 & 149&5.98 & \\
          \textbf{Train} & 5901 & 187& 73&  149&6.02 & \\
          \textbf{Dev} & 59 & 122 & 53 & 102& 6.16 \\
          \textbf{Test} & 1549 & 97 & 45 & 78& 5.83 \\
            \hline
            \multicolumn{7}{c}{\textbf{Pri-NLICE}} \\
          \hline
           {\textbf{Dataset Split}} &  {\textbf{Instances}} & {\textbf{Symptom Type}} & {\textbf{Diagnosis Type}} & {\textbf{Privacy Symptom Type}} &
          {\textbf{Avg. Privacy Symptoms}}\\
          \hline
          \textbf{All} & 3992& 80 &47 & 70&3.76 & \\
          \textbf{Train} & 3168 & 80& 47&  65&3.50 & \\
          \textbf{Dev} & 32 & 50 & 44 & 41& 3.78 \\
          \textbf{Test} & 792 & 43 & 47 & 25& 4.79 \\

          \bottomrule \\
          
        \end{tabular}
    }
    \caption{The statistics of Pri-Ddxplus and Pri-NLICE. Each instance represents a patient's description of symptoms along with the correct diagnosis. Average privacy symptoms indicate the average symptoms occur in one query. }
    \label{tbl:statistics}
\end{table}
